# Supplementary material for: Generalized Similarity U: A Non-parametric Test of Association Based on Similarity
Source: arXiv:1801.01220 ancillary file (2018-01-04)
Supplement: Supplementary file 1 [file Supplementary_material_GSU.pdf]

# Supplementary Materials for: A Generalized Association Test Based on U statistics

**Changshuai Wei**
Department of Biostatistics and Epidemiology,
University of North Texas Health Science Center,
Fort Worth, Texas, USA
changshuai.wei@unthsc.edu

**Qing Lu**
Department of Epidemiology and Biostatistics,
Michigan State University,
East Lansing, Michigan, USA.
qlu@epi.msu.edu

## Supplementary Appendices

### Appendix S1: Centered Similarity

By the following definition of centered similarity,

$$\begin{aligned}\tilde{h}(y_1, y_2) &= h(y_1, y_2) - E(h(y_1, Y_2)) \\ &\quad -E(h(Y_1, y_2)) + E(h(Y_1, Y_2)),\end{aligned}$$

we can obtain conditional expectation for the centered response similarity,

$$\begin{aligned}E(\tilde{h}(Y_1, Y_2)|Y_1) &= E(h(Y_1, Y_2|Y_1)) - E(h(Y_1, Y_2|Y_1)) \\ &\quad -E(h(Y_1, Y_2)) + E(h(Y_1, Y_2)) \\ &= 0.\end{aligned}$$

Therefore, we have $E(\tilde{h}(Y_1, Y_2)) = 0$ and $Var(E(\tilde{h}(Y_1, Y_2)|Y_1)) = 0$. Using the same argument, we can have the same result for the centered predictor similarity.

Denote the function $h_1(y) = E(h(y, Y))$ and the constant $C_h = E(h(Y_1, Y_2))$, the centered similarity can be considered as taking a shift operation on the original similarity,

$$\tilde{h}(y_1, y_2) = h(y_1, y_2) - h_1(y_1) - h_1(y_2) + C_h,$$

so that the resulting similarity has zero mean and zero conditional mean.

In addition, let $\mu_U = E(\tilde{f}(G_1, G_2)\tilde{h}(Y_1, Y_2))$ and $\vartheta = P_{GY} - P_G P_Y$. We can show that

$$\begin{aligned}\mu_U &= \int\int \tilde{f}(g_1, g_2)\tilde{h}(y_1, y_2) dP_{GY}(g_1, y_1) dP_{GY}(g_2, y_2) \\ &= \int\int \tilde{f}(g_1, g_2)\tilde{h}(y_1, y_2) d\vartheta(g_1, y_1) d\vartheta(g_2, y_2) \\ &= \int\int [f(g_1, g_2) - f_1(g_1) - f_2(g_2) + C_f] \\ &\quad \times [h(y_1, y_2) - h_1(y_1) - h_1(y_2) + C_h] d\vartheta(g_1, y_1) d\vartheta(g_2, y_2) \\ &= \int\int f(g_1, g_2) h(y_1, y_2) d\vartheta(g_1, y_1) d\vartheta(g_2, y_2)\end{aligned}$$

where we used the fact that $\int d(P_{G|Y} - P_G) = 0$, $\int d(P_{Y|G} - P_Y) = 0$ and $\int d(P_{GY} - P_G P_Y) = 0$.

## Appendix S2: embedding into Hilbert Space

A Hilbert space $\mathcal{H}$ is a vector space of functions $\varphi : \Psi \to \mathbb{C}$ endowed with an inner product, $< \cdot, \cdot >_{\mathcal{H}}$. Here, we only consider $\mathcal{H}$ of real valued functions, i.e., $\varphi : \Psi \to \mathbb{R}$. We can relate the positive definite kernel with a Hilbert space by the following propositions.

Proposition 1 (proposition 8.5 in Benyamini and Lindenstrauss (1998) ): The kernel $h(y_1, y_2)$ on $\Psi_Y$ is positive definite if only if there is a Hilbert space $\mathcal{H}$ and a map $\tau_h : \Psi_Y \to \mathcal{H}$, s.t., $h(y_1, y_2) =< \tau_h(y_1), \tau_h(y_2) >_{\mathcal{H}} \forall\ y_1, y_2 \in \Psi_Y$.

For each positive definite kernel $h$, we can construct a unique reproducing kernel Hilbert space (RKHS) $\mathcal{H}$ with reproducing kernel $h$ (Berlinet and Thomas-Agnan, 2011), such that, 1) $\forall y \in \Psi_Y$, $h(\cdot, y) \in \mathcal{H}$, 2) $\forall y \in \Psi_Y$, $\forall \varphi \in \mathcal{H}$, $< \varphi, h(\cdot, y) >_{\mathcal{H}} = \varphi(y)$. Be noted here we have $h(\cdot, y) = \tau_h(y)$.

We can represent a measure $\vartheta \in \mathcal{M}$ as an element in RKHS using an embedding map $\pi$: $\mathcal{M} \to \mathcal{H}$, s.t.,

$$\pi_h(\vartheta) = \int \tau_h(y) d\vartheta(y) = \int h(., y) d\vartheta(y).$$

For strongly positive definite kernel $h$, the mapping $\pi_h$ is one-to-one, i.e., $\vartheta_1 = \vartheta_2 \Leftrightarrow \pi(\vartheta_1) = \pi(\vartheta_2)$. "$\Rightarrow$" is obvious. To prove "$\Leftarrow$", observe that $\int\int h(y_1, y_2) d\vartheta(y_1) d\vartheta(y_2) = \int\int < h(\cdot, y_1), h(\cdot, y_2) >_{\mathcal{H}} d\vartheta(y_1) d\vartheta(y_2) = ||\pi(\vartheta)||^2_{\mathcal{H}}$. Thus, $\pi(\vartheta) = 0$ implies $\int\int h(y_1, y_2) d\vartheta(y_1) d\vartheta(y_2) = 0$, which further implies $\vartheta = 0$.

Let $f \otimes h$: $(\Psi_G \times \Psi_Y) \times (\Psi_G \times \Psi_Y) \to R$ be a kernel such that $(f \otimes h)\big((g_1, y_1), (g_2, y_2)\big) = f(g_1, g_2) h(y_1, y_2)$. If $f$ and $g$ are positive definite kernel, then $f \otimes g$ is also positive definite kernel (Hofmann *et al.*, 2008). Thus, there exist a unique RKHS with reproducing kernel $f \otimes h$.

Let $\tau_h(y) = h(\cdot, y)$ and $\tau_f(g) = f(\cdot, g)$. We can then write $\mu_U$ as:

$$\begin{aligned}\mu_U =& \int\int (f \otimes h)\big((g_1, y_1), (g_2, y_2)\big) d\vartheta(g_1, y_1) d\vartheta(g_2, y_2)\\ =& \int\int < \tau_f(g_1)\tau_h(y_1), \tau_f(g_2)\tau_h(y_2) >_{\mathcal{H}} d\vartheta(g_1, y_1) d\vartheta(g_2, y_2)\\ =& ||\pi_{f\otimes h}(\vartheta)||^2_{\mathcal{H}},\end{aligned}$$

where, $\pi_{f\otimes h}$ is a measure embedding s.t.,

$$\pi_{f\otimes h}(\vartheta) = \int\int \tau_f(g)\tau_h(y) d\vartheta(g, y).$$

If $\mu_U = 0$, then we know $\pi_{f\otimes h}(\vartheta) = 0$, i.e.,

$$\int f(g_1, g) h(y_1, y) d\vartheta(g_1, y_1) = 0,\ \forall (g, y) \in \Psi_G \times \Psi_Y.$$

Then we can show the independence $G \perp\!\!\!\perp Y$ by repeatedly using measure embedding (Lyons, 2013). Define a measure $\rho_g$ on $\Psi_Y$, such that $\rho_g(B) = \int f(g_1, g) 1_B(y_1) d\vartheta(g_1, y_1)$, $\forall\ B \subset \Psi_Y$. Then, the measure embedding of $\rho_g$ is $\pi_h(\rho_g) = \int h(y_1, \cdot) f(g_1, g) d\vartheta(g_1, y_1) = 0$, which further implies that $\rho_g = 0$ ($\forall g \in \Psi_G$), i.e., $\int f(g_1, \cdot) 1_B(y_1) d\vartheta(g_1, y_1) = 0$. We further define a measure $\varrho_B$ on $\Psi_G$, such that $\varrho_B(A) = \int 1_A(g_1) 1_B(y_1) d\vartheta(g_1, y_1)$, $\forall A \subset \Psi_G$. Then, the measure embedding of $\varrho_B$ is $\pi_f(\varrho_B) = \int f(g_1, \cdot) 1_B(y_1) d\vartheta(g_1, y_1) = 0$, which further implies that $\varrho_B = 0$. By the definition of $\varrho_B$, we know that,

$$\int 1_A(g_1) 1_B(y_1) d\vartheta(g_1, y_1) = 0, \forall A \subset \Psi_G, \forall B \subset \Psi_Y$$

i.e., $\vartheta = 0$. Thus, $G \perp\!\!\!\perp Y$.

## Appendix S3: Proof of Theorem 3

We can decompose the centered response similarity by, $\tilde{h}(y_1, y_2) = \sum_{s=1}^{\infty} \lambda_s \phi_s(y_1)\phi_s(y_2)$, where $\{\lambda_s\}$ and $\{\phi_s(\cdot)\}$ are eigenvalues and eigenfunctions of the kennel $\tilde{h}(\cdot\,,\cdot)$. Because of the orthogonality of $\{\phi_s(\cdot)\}$ , we have $E(\tilde{h}(Y_1, Y_2)\phi_{s'}(Y_2)|Y_1) = \sum_{s=1}^{\infty} \lambda_s \phi_s(Y_1) \int \phi_s(y_2)\phi_{s'}(y_2)dF(y_2) = \lambda_{s'}\phi_{s'}(Y_1)$. We showed $E(\tilde{h}(Y_1, Y_2) \times 1|Y_1) = 0 \times 1$ in Supplementary Appendix S1, which forced $\phi_1(\cdot) = 1$ and $\lambda_1 = 0$ to be an eigenfunction-eigenvalue pair in the decomposition of $\tilde{h}(\cdot\,,\cdot)$. Again, because $\phi_1(\cdot)$ is orthogonal with $\{\phi_s(\cdot)\}_{s>1}$, for $s > 1$, we have $E\phi_s(Y_1) = \int \phi_s(y_1)\phi_1(y_1)dF(y_1) = 0$. Using the same argument, we have the corresponding results (i.e., $E\varphi_t(G_1) = 0$, $\forall\ t > 1$) for the decomposition of the centered predictor similarity, $\tilde{f}(G_i, G_j) = \sum_{t=1}^{\infty} \eta_t \varphi_t(g_1)\varphi_t(g_2)$. Then,

$$\begin{cases} E\phi_s(Y) = 0, & \forall\, s > 1 \\ E\varphi_t(G) = 0 & \forall\, t > 1. \end{cases} \tag{Ax.1}$$

Using the function decomposition, we can write GSU as,

$$\begin{aligned} U &= \frac{1}{n(n-1)} \sum_{t=1}^{\infty} \eta_t \sum_{s=1}^{\infty} \lambda_s \sum_{i \neq j} \varphi_t(G_i)\varphi_t(G_j)\phi_s(Y_i)\phi_s(Y_j) \\ &= \frac{1}{n-1} \sum_{t=2}^{\infty} \eta_t \sum_{s=2}^{\infty} \lambda_s \left( \frac{1}{\sqrt{n}} \sum_{i=1}^{n} \varphi_t(G_i)\phi_s(Y_i) \right)^2 \\ &\quad - \frac{1}{n-1} \sum_{t=2}^{\infty} \eta_t \sum_{s=2}^{\infty} \lambda_s \frac{1}{n} \sum_{i=1}^{n} (\varphi_t(G_i)\phi_s(Y_i))^2 \\ &= \frac{1}{n-1} \sum_{t=2}^{\infty} \sum_{s=2}^{\infty} \left( \frac{1}{\sqrt{n}} \sum_{i=1}^{n} \eta_t^\star(G_i)\phi_s^\star(Y_i) \right)^2 \\ &\quad - \frac{1}{n-1} \sum_{t=2}^{\infty} \sum_{s=2}^{\infty} \frac{1}{n} \sum_{i=1}^{n} (\eta_t^\star(G_i)\phi_s^\star(Y_i))^2 , \end{aligned}$$

where $\varphi_t^\star(G_i) = \eta_t^{0.5}\varphi_t(G_i)$ and $\phi_s^\star(Y_i) = \lambda_s^{0.5}\phi_s(Y_i)$.

Under the null hypothesis, predictor element $(G_i)$ is independent of response element $(Y_i)$. Therefore, for $s > 1$ and $t > 1$,

$$E(\eta_t^\star(G_1)\phi_s^\star(Y_1)) = \eta_t^{0.5} E\varphi_t(G_1)\lambda_s^{0.5} E\phi_s(Y_1) = 0, \tag{Ax.2}$$

and

$$E(\eta_t^\star(G_1)\phi_s^\star(Y_1)\eta_{t'}^\star(G_1)\phi_{s'}^\star(Y_1)) = \begin{cases} \eta_t\lambda_s, & \text{if } s = s' \text{and } t = t' \\ 0, & \text{otherwise.} \end{cases} \tag{Ax.3}$$

Therefore, for any finite subset $\Delta$ of $\{(s, t)\}_{s>1,t>1}$, the multivairate random variables $\left\{ \frac{1}{\sqrt{n}} \sum_{i=1}^{n} \eta_t^\star(G_i)\phi_s^\star(Y_i) \right\}_{(s,t)\in\Delta}$ converges to a multivariate normal distribution by using results from equation Ax.2, equation Ax.3 and multivariate CLT. Additionally, we can show that,

$$\begin{aligned} \sum_{s>1,t>1} E(\eta_t^\star(G_1)\phi_s^\star(Y_1))^2 =& \sum_{s} \lambda_s \sum_{t} \eta_t \\ =& E(h(Y, Y))E(f(G, G)) < \infty. \end{aligned}$$

Under the condition $\sum_{s>1,t>1} E(\eta_t^\star(G_1)\phi_s^\star(Y_1))^2 < \infty$, the infinite countable sequence of function $\{\eta_t^\star(\cdot)\phi_s^\star(\cdot)\}$ is a Donsker class (Theorem 2.13.1 in van der Vaart and Wellner (2000)). Therefore, the empirical process, $\frac{1}{\sqrt{n}} \sum_{i=1}^{n} \eta_t^\star(G_i)\phi_s^\star(Y_i)$, converges weakly to the Gaussian process $Z_{s,t}$ with mean zero and covariance function, $cov(Z_{s,t}, Z_{s',t'}) = E(\eta_t^\star(G_1)\phi_s^\star(Y_1)\eta_{t'}^\star(G_1)\phi_{s'}^\star(Y_1))$. With this uniform convergence (for all $s > 1$ and $t > 1$), we can show that,

$$nU \xrightarrow{D} \sum_{t=2}^{\infty} \sum_{s=2}^{\infty} (Z_{s,t})^2 - \sum_{t=2}^{\infty} \sum_{s=2}^{\infty} \eta_t\lambda_s = \sum_{t=1}^{\infty} \eta_t \sum_{s=1}^{\infty} \lambda_s(\chi_{st}^2 - 1),$$

where $\chi_{st}^2$ are i.i.d chi-squared random variables with a d.f. of 1.

## Appendix S4: Proof of Theorm 4

To simplify the notation, we denote $X = (Y, G)$ and $u(X_1, X_2) = \tilde{f}(G_1, G_2)\tilde{h}(Y_1, Y_2)$. GSU can then be rewritten as:

$$U = \frac{1}{n(n-1)} \sum_{i \neq j} u(X_i, X_j).$$

Define a centered kernel $\tilde{u}(x_1, x_2)$ by:

$$\tilde{u}(x_1, x_2) = u(x_1, x_2) - u_1(x_1) - u_1(x_2) - \mu,$$

where $u_1(x) = E(u(X_1, X_2)|X_1 = x)$.

We can decompose the GSU as follows:

$$\begin{aligned} U &= \frac{1}{n(n-1)} \sum_{i \neq j} u(X_i, X_j) \\ &= \frac{1}{n(n-1)} \sum_{i \neq j} (\tilde{u}(X_i, X_j) + u_1(X_i) + u_1(X_j) - \mu) \\ &= \frac{1}{n(n-1)} \sum_{i \neq j} \tilde{u}(X_i, X_j) + \frac{2}{n} \sum_{i=1}^{n} (u_1(X_i) - \mu) + \mu. \end{aligned}$$

Thus,

$$\sqrt{n}(U - \mu) = \frac{2}{\sqrt{n}} \sum_{i=1}^{n} (u_1(X_i) - \mu) + \frac{\sqrt{n}}{n(n-1)} \sum_{i \neq j} \tilde{u}(X_i, X_j).$$

Becuase $E(u_1(X)) = \mu$ and $Var(u_1(X)) = \zeta_1$, the first term converges to normal distribution by applying CLT:

$$\frac{2}{\sqrt{n}} \sum_{i=1}^{n} (u_1(X_i) - \mu) \xrightarrow{D} N(0, 4\zeta_1).$$

Then we need to show:

$$R = \frac{\sqrt{n}}{n(n-1)} \sum_{i \neq j} \tilde{u}(X_i, X_j) \xrightarrow{p} 0.$$

This can be done by proving $ER^2 \to 0$, using the fact that $E(\tilde{u}(X_1, X_2)) = 0$, $Var(\tilde{u}(X_1, X_2)) < \infty$ and $E(\tilde{u}(X_1, X_2)|X_1) = 0$. In fact, by using the similar technique in Appendix B, we can show that $\sqrt{n}R$ asymptotically follows the distribution of a weighted sum of independent chi-square random variables.

## Appendix S5: Matrix Similarity

In the study sample, we can calculate the centered phenotype similarity by:

$$\begin{aligned} \tilde{h}(y_i, y_j) =& h(y_i, y_j) - \frac{1}{n} \sum_{j=1}^{n} h(y_i, y_j) \\ & - \frac{1}{n} \sum_{i=1}^{n} h(y_i, y_j) + \frac{1}{n^2} \sum_{i,j} h(y_i, y_j). \end{aligned}$$

Denote $\tilde{S}_{i,j} = \tilde{h}(y_i, y_j)$ and $S_{i,j} = h(y_i, y_j)$, the above equation becomes:

$$\tilde{S}_{i,j} = S_{i,j} - \frac{1}{n} \sum_{j=1}^{n} S_{i,j} - \frac{1}{n} \sum_{i=1}^{n} S_{i,j} + \frac{1}{n^2} \sum_{i,j} S_{i,j}.$$

The equations can be written in a matrix form,

$$\begin{aligned} \tilde{S} &= S - JS - SJ + JSJ \\ &= (I - J)S(I - J), \end{aligned}$$

where $\tilde{S} = \{\tilde{h}(y_i, y_j)\}_{n\times n}$, $S = \{h(y_i, y_j)\}_{n\times n}$, $I = \{1_{\{i=j\}}\}_{n\times n}$, and $J = \{\frac{1}{n}\}_{n\times n}$. Similarly, the centered genetic similarity can also be written in the matrix form:

$$\tilde{K} = (I - J)K(I - J),$$

where $\tilde{K} = \{\tilde{f}(g_i, g_j)\}_{n\times n}$, and $K = \{f(g_i, g_j)\}_{n\times n}$.

## Appendix S6: Covariate Adjustment

The rational here is to obtain a covariate-centered similarity, so that the centered similarity is perpendicular to the space spanned by the covariates. We first consider the phenotype similarity and assume the covariates to be a $P + 1$ dimensional function: $x_i = x(y_i)$. We define a new kernel by:

$$u(y_1, y_2) = x(y_1)\Big[E\big(x(\cdot)^T x(\cdot)\big)\Big]^{-1} x(y_2)^T.$$

From this definition, we have,

$$E(u(y_1, Y_2)x(Y_2)) = x(y_1).$$

The covariate-centered kernel is then defined as:

$$\begin{aligned}\hat{h}(y_1, y_2) =& \tilde{h}_0(y_1, y_2) - E[\tilde{h}_0(y_1, Y_3)u(Y_3, y_2)] \\ & - E[u(y_1, Y_3)\tilde{h}_0(Y_3, y_2)] \\ & + E[u(y_1, Y_3)\tilde{h}_0(Y_3, Y_4)u(Y_4, y_2)].\end{aligned}$$

With this definition, we can show that,

$$\begin{aligned}& E[\hat{h}(y_1, Y_2)x(Y_2)] \\ =& \int \tilde{h}_0(y_1, y_2)x(y_2)dF(y_2) \\ & - \int\int \tilde{h}_0(y_1, y_3)E\Big[u(y_3, Y_2)x(Y_2)\Big]dF(y_3) \\ & - \int\int u(y_1, y_3)\tilde{h}_0(y_3, y_2)x(y_2)dF(y_3)dF(y_2) \\ & + \int\int u(y_1, y_3)\tilde{h}_0(y_3, y_4)E\Big[u(y_4, Y_2)x(Y_2)\Big]dF(y_4)dF(y_3) \\ =& 0.\end{aligned}$$

Consider the above expectation as an inner product,

$$< \hat{h}(\cdot, y_2), x(y_2) >= \int \hat{h}(\cdot, y_2)x(y_2)dF(y_2).$$

Then, $< \hat{h}(\cdot, y_2), x(y_2) >= 0$ means $\hat{h} \perp x$, i.e., the new similarity $\hat{h}$ is perpendicular to the space spanned by the covariates.

In the study sample, we can compute covariate-centered similarity by replacing the expectation with a sample average,

$$\begin{aligned}& \hat{h}(y_i, y_j) \\ =& \tilde{h}_0(y_i, y_j) - \sum_{k=1}^{n} x_i(\sum_{l=1}^{n} x_l^T x_l)^{-1} x_k^T \tilde{h}_0(y_k, y_j) \\ & - \sum_{k=1}^{n} \tilde{h}_0(y_i, y_k)x_k(\sum_{l=1}^{n} x_l^T x_l)^{-1} x_j^T \\ & + \sum_{m=1}^{n}\sum_{k=1}^{n} x_i(\sum_{l=1}^{n} x_l^T x_l)^{-1} x_m^T \tilde{h}_0(y_m, y_k)x_k(\sum_{l=1}^{n} x_l^T x_l)^{-1} x_j^T.\end{aligned}$$

As in Appendix E, this can be written as a matrix form,

$$\hat{S} = (I - X(X^T X)^{-1} X^T)\tilde{S}_0(I - X(X^T X)^{-1} X^T).$$

Similarly, the covariate centered genetic similarity can be computed by,

$$\hat{K} = (I - X(X^T X)^{-1} X^T)\tilde{K}_0(I - X(X^T X)^{-1} X^T).$$

## Appendix S7: Limiting Distribution

In the actual computation, we will use a matrix eigen-decomposition to obtain the eigenvectors as a finite-dimension approximation of the eigenfunctions. For a matrix eigen-decomposition, a computer algorithm usually gives the eigenvalue $\lambda_s$ with the eigenvector $\phi_s$, which satisfies $\sum_{i=1}^n \phi_{s,i}^2 = 1$ instead of $\frac{1}{n}\sum_{i=1}^n \phi_{s,i}^2 = 1$. Therefore, using the eigenvalues $\hat{\lambda}_s$ and $\hat{\eta}_t$ calculated from the matrix eigen-decomposition, the limiting distribution of GSU is:

$$n\hat{U} \sim \frac{n}{n-P-1}\sum_{t=1}^{n}\frac{\hat{\eta}_t}{n}\sum_{s=1}^{n}\frac{\hat{\lambda}_s}{n}\chi_{st}^2,$$

where, the factor $\frac{n}{n-P-1}$ is added in the calculation to take into account of the projection operator $I - X(X^T X)^{-1} X^T$ for finite sample.

## Appendix S8: Simulation I, II and III

1. *Simulation I Setting.* The null models were simulated by setting $\mu_\beta = 0$ and $\sigma_\beta^2 = 0$. For the alternative, two sets of models were simulated:

   (a) $\mu_\beta = 0$ and $\sigma_\beta^2 > 0$ so that half of the causal SNVs were deleterious and the other half were protective.

   (b) $\mu_\beta > 0$ and $\sigma_\beta^2 > 0$ so that majority of the causal SNVs were deleterious.

   The details of the simulation setting can be found in Table S1 of Supplementary Materials.

2. *Simulation II Setting.* We allow the multivariate phenotype to contain variables that follow different distributions. In particular, we simulated 4 combinations:

   (a) 1 binary-distributed variable and 2 Poisson-distributed variables, denoted as BPP;

   (b) 1 Cauchy-distributed variables and 2 Gaussian-distributed variables, denoted as CGG;

   (c) 2 binary-distributed variables and 1 Gaussian-distributed variable, denoted as BBG;

   (d) 1 binary-distributed variable, 1 Gaussian distributed variable and 1 Cauchy distributed variable, denoted as BGC.

   The setting is chosen so that we have 1 multivariate phenotype of only categorical variables (i.e., BPP), 1 multivariate phenotype of only continuous variables (i.e., CGG) and 2 multivariate phenotypes with mixture of continuous and categorical variables (i.e., BBG and BCG). For the null model, we set $\mu_\beta = 0$ and $\sigma_\beta^2 = 0$ . For the alternative models, we set $\mu_\beta = 0$ and $\sigma_\beta^2 > 0$ , and allowed the multiple phenotypes to be influenced by different sets of causal SNVs. The details of the simulation setting were described in Table S2 of Supplementary Materials.

3. *Simulation III Setting.* To simulate confounding effects, we first generated a covariate vector, $x_i = (x_{1,i}, x_{2,i})^T$, where, $x_{1,i}$ is a continuous variable, $x_{2,i}$ is a binary variable and both of them are correlated with the SNV-set $g_i$. For the simulation of phenotype, we set $\mu_i = x_i^T\alpha$, where $\alpha$ is the effect vector for the covariates. Given $\mu_i$, we generated multivariate phenotypes, BPP, CGG, BBG, and BGC, in the same way as Simulation II. The details of the simulation setting were in Table S3.

   (a) For the null model, we set $\mu_\beta = 0$ and $\sigma_\beta^2 = 0$. We investigate the type I error rates of the methods with and without adjusting for the confounding variables.

   (b) For the alternative models, we set $\mu_\beta = 0$ and $\sigma_\beta^2 > 0$. We investigated the power of the methods by varying $n$ from 50 to 200.

## Appendix S9: Simulation IV

In this set of simulation, we generate dependence structure via rotation. We first generate one multimodal continuous variable $Y'$,

$$Y' = X_1 + X_2 + X_3,$$

where $X_1 \sim unif(-0.05, 0.05)$, $X_2 \sim (1, 0.5)$, and $X_3 \sim B(1, 0.5)$. We then generate a second variable $G'$ in the same manner (i.i.d copy of $Y'$). Consider $(Y', G')$ as a random vector, we generate another vector $(Y, G)$ by rotating the vector $(Y', G')$ with an angel $\theta \in (0, \pi/4)$,

$$\begin{cases} Y = cos(\theta)G' - sin(\theta)Y', \\ G = cos(\theta)G' + sin(\theta)Y'. \end{cases}$$

For each observation $i$, we generate three pairs of rotated vectors so as to form a response vector $Y_i = (Y_{i1}, Y_{i2}, Y_{i3})$ and a predictor vector $G_i = (G_{i1}, G_{i2}, G_{i3})$. For this simulation, we set the rotation angel as $\pi/5$. We plot the null model ($\theta = 0$) and the alternative model ($\theta = \pi/5$) in Figure S3.

The simulation results were plotted in Figure S4 for different sample sizes. For null model, both GSU and VCscore can correctly control type I error. For alternative model, power of GSU was 0.698 for sample size 50 and increased to 1 for sample size 100 and 200. However, VCscore was unable to detect the association.

# References


Benyamini, Y. and Lindenstrauss, J. (1998). *Geometric nonlinear functional analysis*, volume 48. American Mathematical Soc.

Berlinet, A. and Thomas-Agnan, C. (2011). *Reproducing kernel Hilbert spaces in probability and statistics*. Springer Science & Business Media.

Hofmann, T., Schölkopf, B., and Smola, A. J. (2008). Kernel methods in machine learning. *The annals of statistics*, pages 1171–1220.

Lyons, R. (2013). Distance covariance in metric spaces. *The Annals of Probability*, **41**(5), 3284–3305.

van der Vaart, A. and Wellner, J. A. (2000). *weak convergence and empirical processes*. Springer, 2 edition.

## Supplementary Tables

Table S1: Simulation settings for simulation I

| **Model*** | **Pct**** | | **Settings for effect** | | | |
|---|---|---|---|---|---|---|
| | | | B | C | G | P |
| $Alt_1$ | 30 | $\sigma_\beta$ | 8 | 4 | 1 | 2 |
| | | $\mu_\beta$ | 0 | 0 | 0 | 0 |
| $Alt_2$ | 30 | $\sigma_\beta$ | 8 | 4 | 1 | 2 |
| | | $\mu_\beta$ | 4 | 2 | 0.5 | 1 |

*percentage of functional SNVs

Table S2: Simulation settings for simulation II

| | **Pct*** | | **Settings for effect** | | | |
|---|---|---|---|---|---|---|
| | | | B | C | G | P |
| Alt | 30 | $\sigma_\beta$ | 4 | 2 | 0.5 | 1 |
| | | $\mu_\beta$ | 0 | 0 | 0 | 0 |

*percentage of functional SNVs

Table S3: Simulation settings for simulation III

| | **Pct*** | | **Settings for effect** | | | |
|---|---|---|---|---|---|---|
| | | | B | C | G | P |
| Alt | 30 | $\sigma_\beta$ | 2 | 1 | 0.25 | 5 |
| | | $\mu_\beta$ | 0 | 0 | 0 | 0 |

*percentage of functional SNVs

Table S4: Type I error and power of VCscore and GSU for the univariate analysis of both common and rare variants

| **Model** | **Method** | **Distributions*** | | | |
|---|---|---|---|---|---|
| | | B | C | G | P |
| Null | VCscore | 0.026 | 0.074 | 0.024 | 0.036 |
| | GSU | 0.042 | 0.054 | 0.04 | 0.056 |
| $Alt_1$ | VCscore | 0.764 | 0.573 | 0.878 | 0.795 |
| | GSU | 0.807 | 0.885 | 0.853 | 0.813 |

*B, C, G, P represent a Binary-distributed, Cauchy distributed, Gaussian-distributed, and Poisson distributed phenotype, respectively.

Table S5: Type I error at different cut-offs for n=200

| **Cut-offs** | **Methods** | **Distributions** | | | |
|---|---|---|---|---|---|
| | | BPP | CGG | BBG | BCG |
| 0.01 | VCscore | 0.017 | 0.179 | 0.021 | 0.179 |
| | GSU | 0.011 | 0.012 | 0.011 | 0.012 |
| 0.005 | VCscore | 0.011 | 0.165 | 0.013 | 0.165 |
| | GSU | 0.0061 | 0.0071 | 0.0059 | 0.0069 |

Table S6: Type I error and power comparisons between VCscore and GSU when the variables in multivariate phenotype have the same distribution

| **Model** | **Method** | **Distributions*** | | | |
|---|---|---|---|---|---|
| | | BBB | CCC | GGG | PPP |
| Null | VCscore | 0.0008 | 0.138 | 0.018 | 0.04 |
| | GSU | 0.058 | 0.056 | 0.052 | 0.056 |
| Alt | VCscore | 0.26 | 0.284 | 0.958 | 0.966 |
| | GSU | 0.862 | 0.724 | 0.882 | 0.862 |

Table S7: Weights for the corresponding 6 phenotypes

| FDG | Hippocampus | Entorhinal | AV45 | Fusiform | Ventricles |
|---|---|---|---|---|---|
| 0.383666 | 0.362734 | 0.21682 | 0.635264 | 0.456543 | 0.03228 |

Table S8: Top 20 association findings from whole genome sequencing analysis of both common and rare variants

| SNV-set | size* | p-value |
|---|---|---|
| APOE | 17 | 2.77E-48 |
| ch19-45389309-45439308 | 162 | 1.64E-37 |
| APOC1 | 37 | 3.38E-31 |
| TOMM40 | 126 | 9.28E-19 |
| RHPN2 | 758 | 2.54E-06 |
| ch7-38020963-38070962 | 404 | 3.86E-06 |
| GOT1 | 212 | 4.63E-06 |
| ch13-40620095-40670094 | 422 | 6.21E-06 |
| ZNF805 | 191 | 8.09E-06 |
| ch1-218213012-218263011 | 276 | 9.72E-06 |
| TMEM127 | 78 | 1.08E-05 |
| PVRL2 | 415 | 1.58E-05 |
| ch2-96910630-96960629 | 36 | 1.58E-05 |
| ch22-47050435-47100434 | 48 | 2.05E-05 |
| KCNA10 | 14 | 2.39E-05 |
| CHRNA4 | 170 | 3.14E-05 |
| SNRNP200 | 125 | 3.70E-05 |
| CBLC | 216 | 4.80E-05 |
| ch12-108860220-108910219 | 366 | 5.70E-05 |
| ch10-67010494-67060493 | 463 | 5.96E-05 |

* Number of SNVs in the SNV-set

Table S9: Top 20 association findings from whole genome sequencing analysis of rare variants

| **SNV-set** | **Size*** | **p-value** |
|---|---|---|
| ch1-107013494-107063493 | 240 | 1.96E-06 |
| APOC1 | 26 | 6.28E-06 |
| ch17-40300052-40350051 | 64 | 2.51E-05 |
| ch4-189560456-189610455 | 314 | 3.14E-05 |
| LOC101927616 | 107 | 3.16E-05 |
| ch20-31160828-31210827 | 72 | 4.02E-05 |
| ch7-55470963-55520962 | 126 | 4.29E-05 |
| ch7-55520963-55570962 | 144 | 6.01E-05 |
| ch2-177610797-177660796 | 300 | 6.09E-05 |
| ch4-188410456-188460455 | 183 | 6.44E-05 |
| ch5-89162267-89212266 | 211 | 7.33E-05 |
| ch4-137010456-137060455 | 253 | 7.70E-05 |
| ch17-70050052-70100051 | 70 | 7.78E-05 |
| USP14 | 267 | 8.03E-05 |
| ch8-60863588-60913587 | 307 | 8.51E-05 |
| LOC102723517 | 113 | 8.62E-05 |
| ch3-100810157-100860156 | 292 | 9.87E-05 |
| ch5-130162267-130212266 | 268 | 9.98E-05 |
| ch6-71308317-71358316 | 260 | 0.000114 |
| VOPP1 | 720 | 0.000114 |

* Number of SNVs in the SNV-set

Table S10: The top association findings using the VCscore method

| **SNV-sets** | **Size*** | **p-value** |
|---|---|---|
| APOE | 17 | 1.98E-26 |
| ch19-45389309-45439308 | 162 | 6.64E-22 |
| APOC1 | 37 | 2.91E-17 |
| TOMM40 | 126 | 2.11E-9 |

* Number of SNVs in the SNV-set

**time for analyze the 4 SNV sets is 147 seconds using VCscore, and 5.2 seconds using GSU

Table S11: The top association findings using the case control status

| **SNV-sets** | **Size*** | **p-value** |
|---|---|---|
| APOE | 17 | 3.44E-08 |
| ch19-45389309-45439308 | 162 | 1.88E-05 |
| APOC1 | 37 | 0.000184 |
| TOMM40 | 126 | 0.007053 |

* Number of SNVs in the SNV-set

Table S12: Type I error at different cut-offs with n=50 for GSU-rk

| **Cut-offs** | **Distributions** | | | |
|---|---|---|---|---|
| | BPP | CGG | BBG | BCG |
| 0.01 | 0.010 | 0.010 | 0.010 | 0.009 |
| 0.005 | 0.0052 | 0.0051 | 0.005 | 0.0049 |
| 0.0005 | 0.00042 | 0.00045 | 0.00042 | 0.00043 |

Table S13: Performance of VCscore and GSU when the Poisson distributions are more right skewed.

| **Model** | **Method** | **PPP** | |
|---|---|---|---|
| | | $\mu = -10$ | $\mu = -3$ |
| Null | VCscore | 0 | 0.116 |
| | GSU | 0 | 0.034 |
| Alt | VCscore | 0.45 | 0.95 |
| | GSU | 0.652 | 0.862 |

* Type I errors is 0 for $\mu = -10$, due to the fact that all the phenotype values are 0 in this particular simulation.

Table S14: Power comparison of VCscore-rk and GSU-rk under different phenotype distributions

| | | Methods | |
|---|---|---|---|
| Distribution | Setting | VCscore-rk | GSU-rk |
| B | Null | 0.007 | 0.057 |
| | Alt | 0.043 | 0.2215 |
| C | Null | 0.03 | 0.054 |
| | Alt | 0.345 | 0.492 |
| G | Null | 0.037 | 0.06 |
| | Alt | 0.307 | 0.285 |
| P | Null | 0.024 | 0.056 |
| | Alt | 0.506 | 0.488 |
| BCG | Null | 0.043 | 0.048 |
| | Alt | 0.275 | 0.413 |

Table S15: Spearman correlations among variables in multivariate phenotype

| **Spearman Correlations for BBG** | | | |
|---|---|---|---|
| | B1 | B2 | G3 |
| B1 | 1 | 0.274 | 0.418 |
| B2 | 0.274 | 1 | 0.420 |
| G3 | 0.418 | 0.420 | 1 |
| **Spearman Correlations for CCP** | | | |
| | C1 | C2 | P3 |
| C1 | 1 | 0.252 | 0.401 |
| C2 | 0.252 | 1 | 0.395 |
| P3 | 0.401 | 0.395 | 1 |

*The correlation is average value of spearman correlations from 1000 simulation replicates.

# Supplementary Figures

Figure S1: Power comparison when the dimension of phenotype is 10

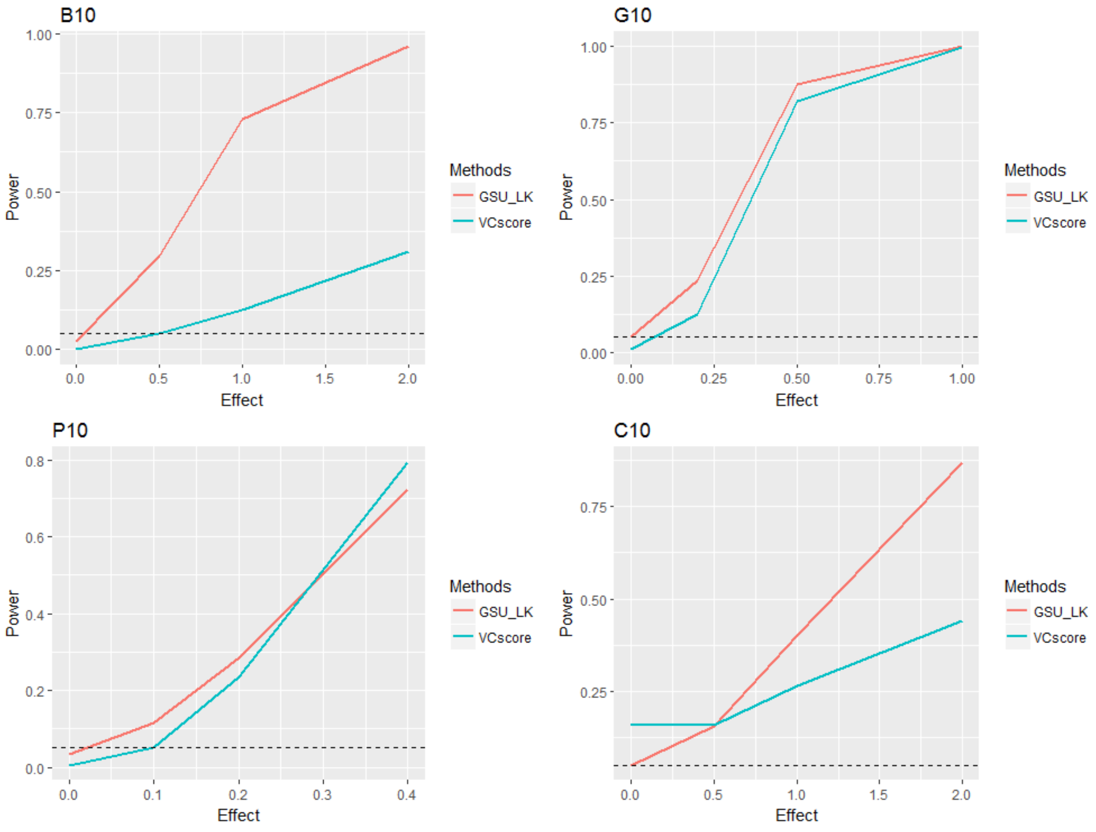


* B10, G10, P10 and C10 represents multivariate phenotype with 10 binary variables, 10 Gaussian variables, 10 Poisson variables and 10 Cauchy variables, respectively.

Figure S2: QQ plot for whole genome sequencing analysis of both common and rare variants.

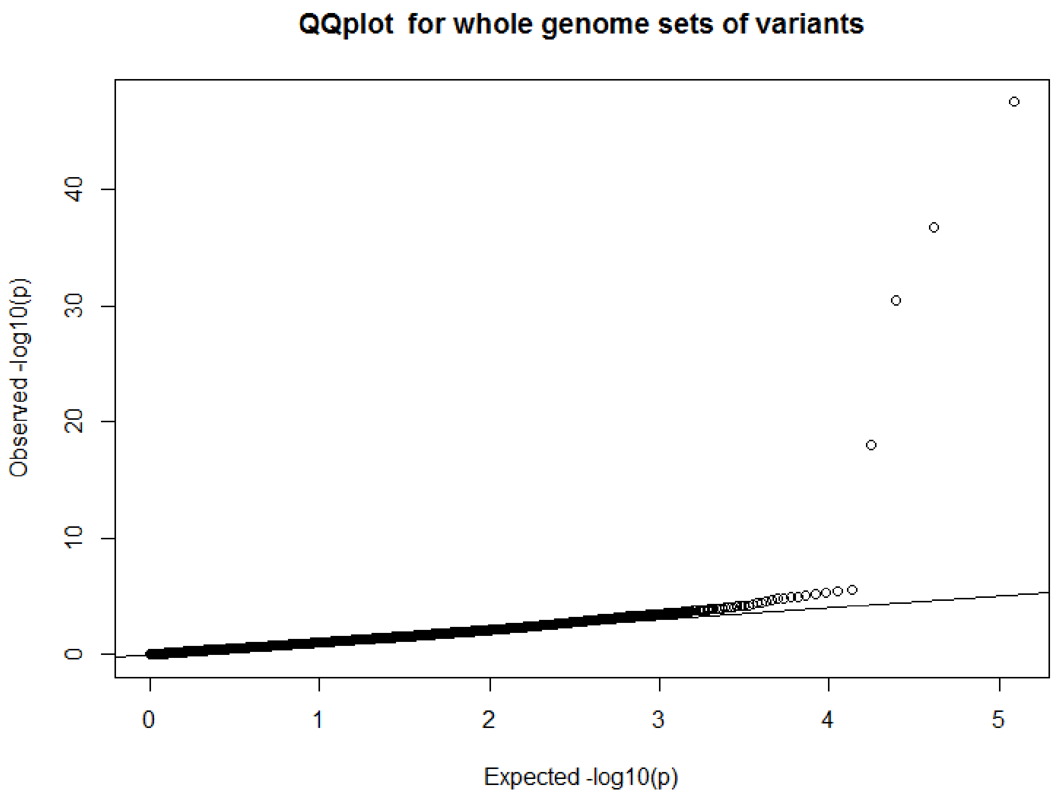

Figure S3: QQ plot for whole genome sequencing analysis of rare variants.

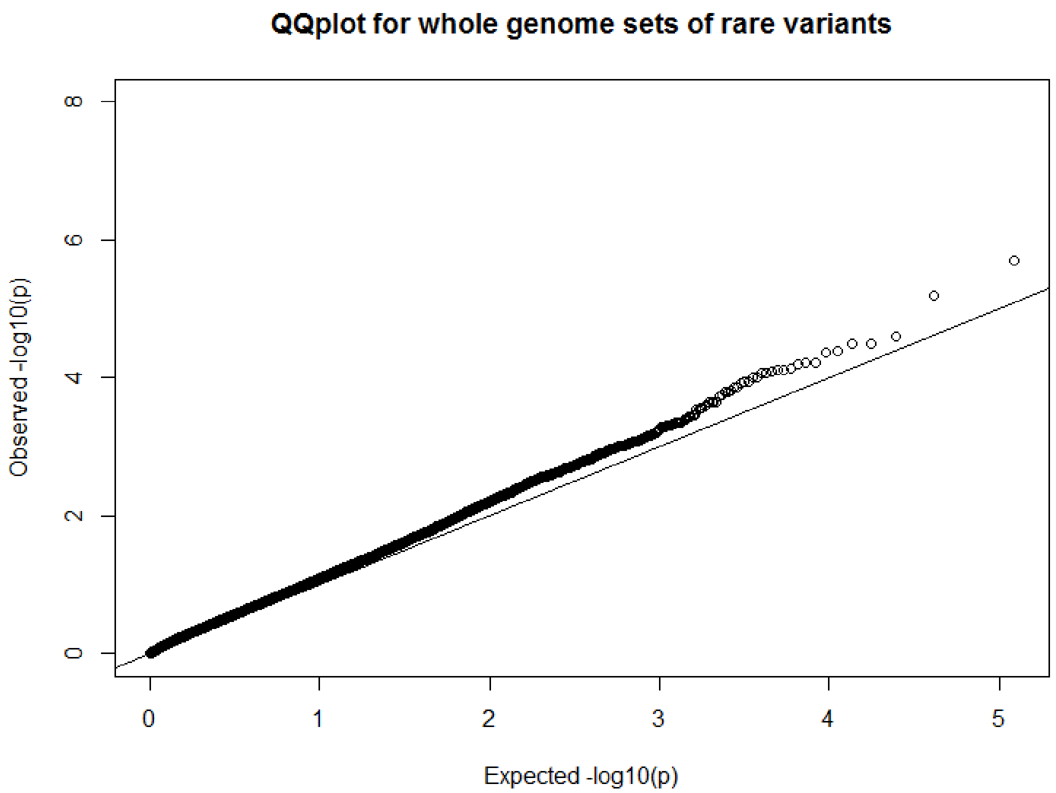

Figure S4: Simulation settings for the rotation model

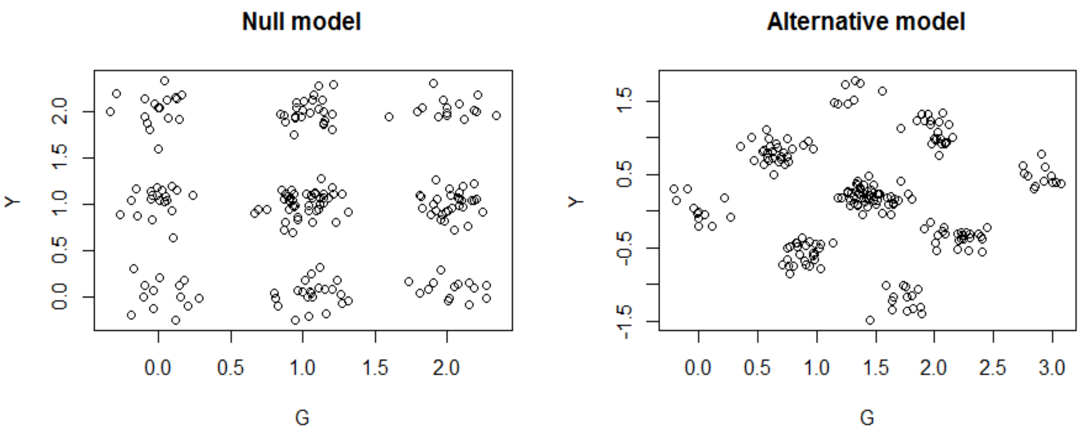


Figure S5: Simulation result for the rotation model

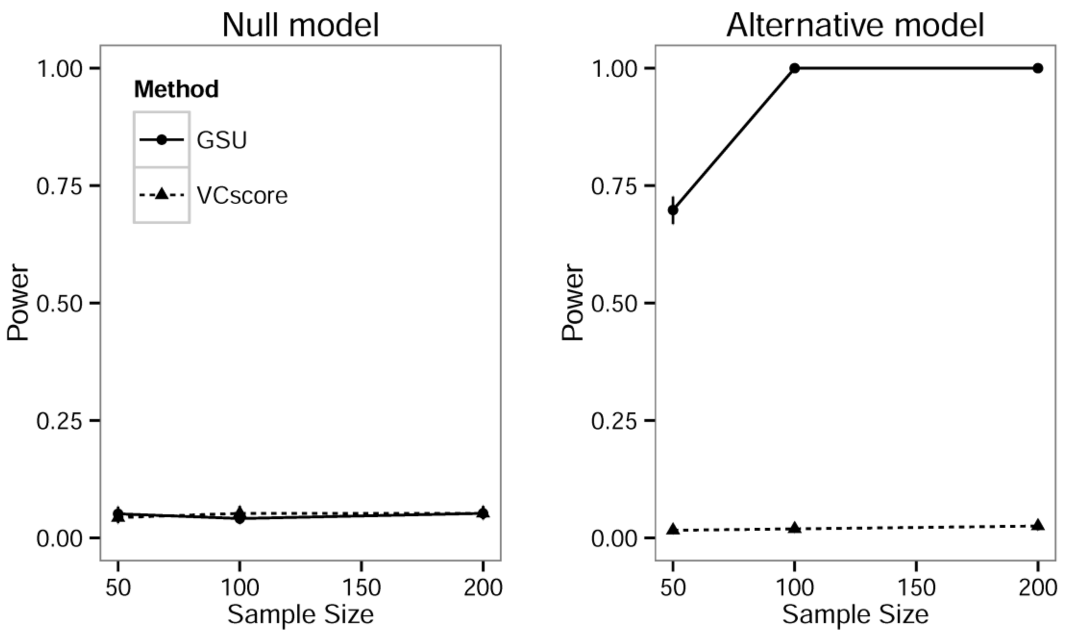

Figure S6: Power comparison for GSU with different kernels and VCscore with the cross product kernel

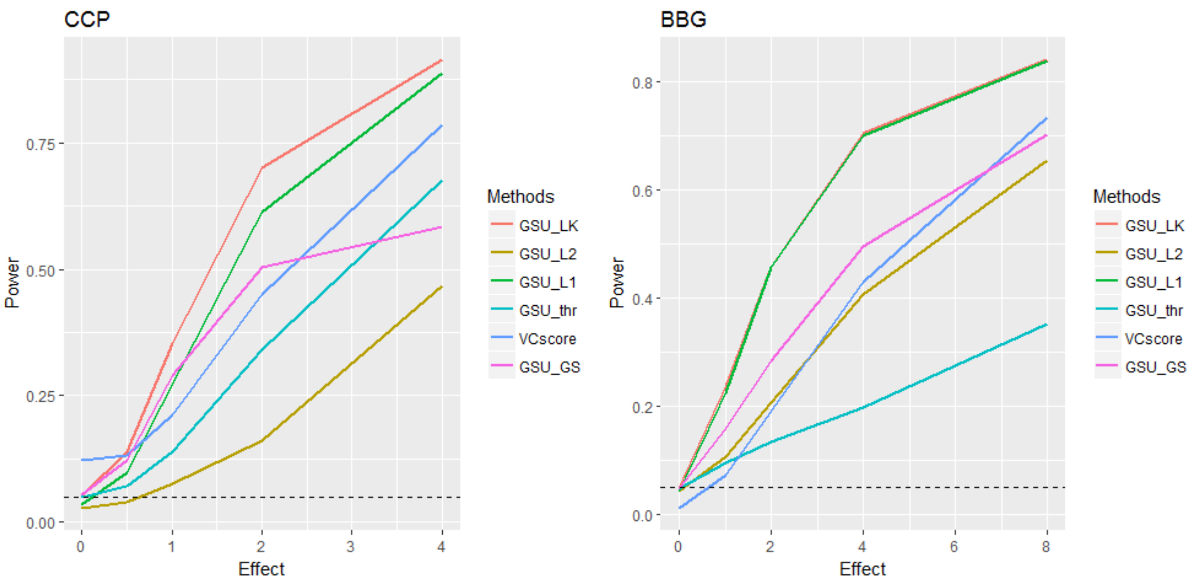


*all methods here use same similarity measurements for both phenotype similarity and genotype similarity

**GSU_LK, GSU_L2, GSU_L1, GSU_thr, and GSU_GS represents GSU with the Laplacian kernel, the negative L2 distance kernel, the negative L1 distance kernel, the thresholding transform of distance kernel, and the Gaussian kernel, respectively. VCscore represents VCscore with the cross product kernel.

***Note that for the CCP phenotype, the power curve for VCscore is not valid, since it cannot control type I error.

****Among these, kernels in GSU_LK, GSU_GS, and GSU_L1 are strongly positive definite kernels.

Figure S7: Tail behavior of GSU for the small and large sample sizes with 1 million null simulation replicates

n=50

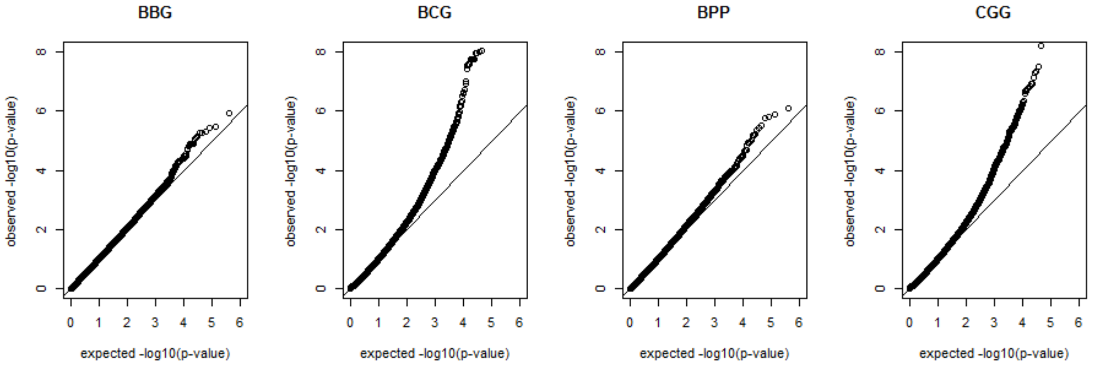


n=500

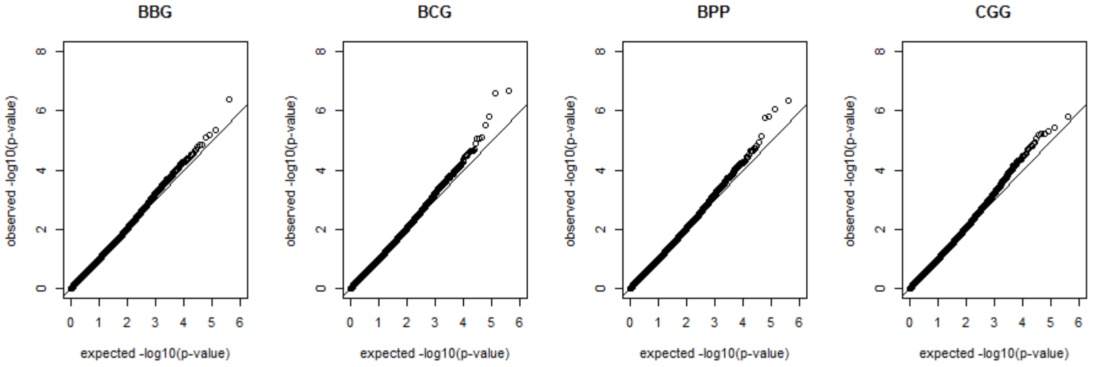

Figure S8: Power curve for GSU when the dimension of phenotype is increased to 100

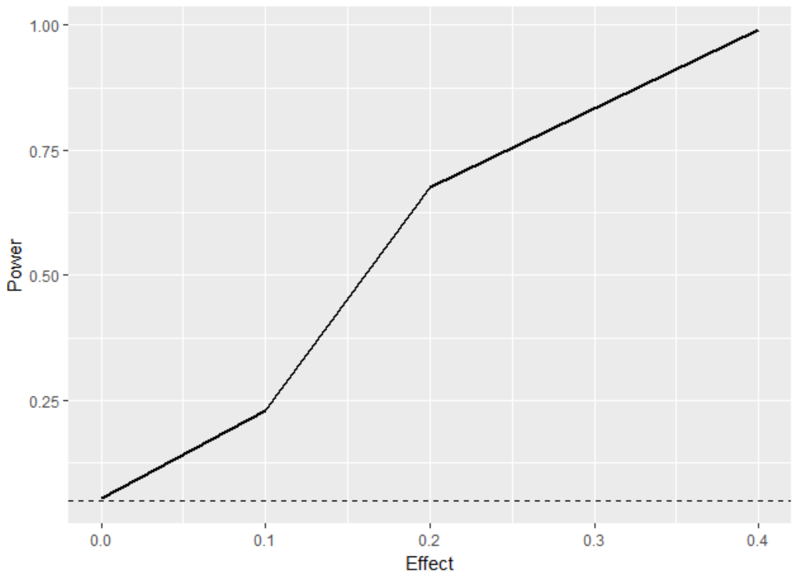

Figure S9: Power comparisons between GSU and VCscore when there are correlations among phenotypes

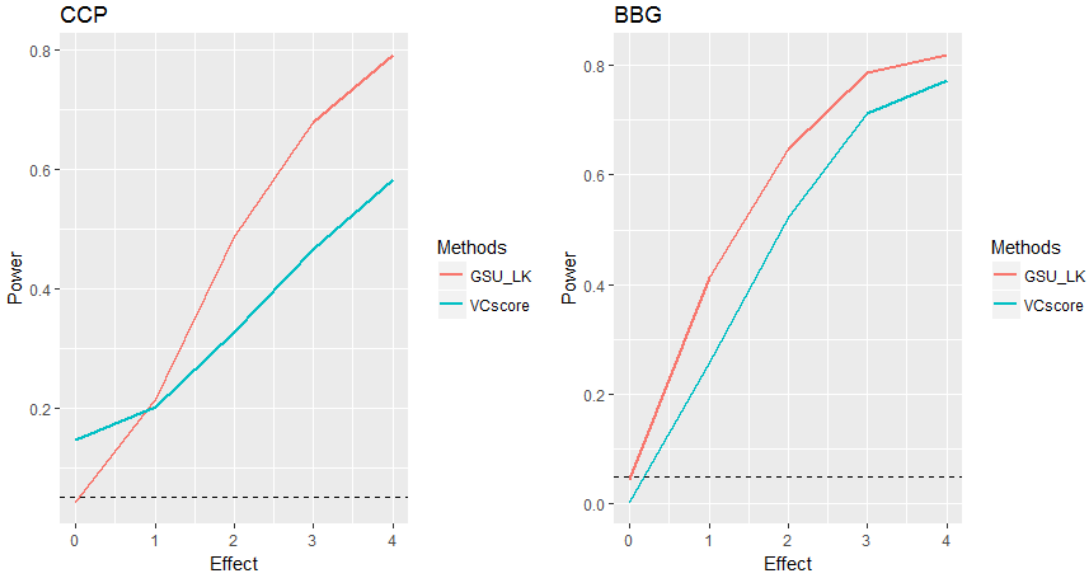


*correlations among phenotype for null effects are summarized in Table S15
